# Supplementary material for: Query-Driven Sampling for Collective Entity Resolution
Source: arXiv:1508.03116 source file (2015-08-13)
Supplement: Supplementary file 1 [file appendix.tex]

\twocolumn

\textbf{Will not be included in sigmod14 version}
 
\appendix

\section{Influence Function Implementation Details}
\label{sec:if_details}

The $\mathcal{I}$ data structure is created using Vose's algorithm~\cite{Vose:1991:LAG:126262.126280}.
Also called the Alias method, this process allows us to build a
data structure in linear time with respect to the number of mentions in the data set.
Practically, creation takes 2 seconds for 1 million mentions with most of the time being feature calculation.
Secondly, the $\mathcal{I}$ samples mentions in proportion to their distance in $\Theta(1)$ time.

This construction algorithm works by inputing mentions and their influence distance to a query node.
Then, probabilities are sliced and fit into two arrays
such that a uniform selection of an item in an array and a biased
coin can be flipped such that a node is selected in proportion to its influence.

We compute the influence distance by computing the pairwise feature scores between the
query node and each other mentions.
The construction of the influence data structure is performed only once and does not change.
We do not compute non-pairwise features when calculating influence because entity-wide
and other entities change during the process of the algorithm.

%[[How we build data structure to sample by influence]]

%[[Explain how we perform the first round of influence in calculation in the database
%so we can ignore low influence mentions.
%Explain that the choice of cutoff can be chosen with respect to memory and the desired
%performance characteristics.]]

In general graphical models, influence between two nodes is calculated by computing the
factors on the active trail between the nodes.
Coreference is a pairwise model, the active trail contains only one factor.
This property makes it extremely efficient to compute influence.

The influence data structure can be constructed in the database while computing and retrieving the canopy.
The path scores are computed and a query entity canopy is created by specifying a threshold where very
small scores are removed from the canopy.
Low influence scores create a natural canopy because all values of low influence mentions will be sampled rarely if at all.
The distribution of these mention influence scores is important to the effectiveness of algorithms.
In the case where the mention influence scores are uniform the sample in Algorithm~\ref{algo:queryproportional}
make it random, and the same as Algorithm~\ref{algo:erbase}.

It is possible that the influence function is too strict.
For example, the mention set may have only a few high scoring mentions and a large number of low scoring mentions.
In such cases, it is still desirable for some of the low scoring mentions to be proposed for merge.
To alleviate this situation we can
vary the distribution of the influence function $\mathcal{I}$ by
fitting the influence function to a curve of our choosing.
We rank pairwise the scores of the nodes over a \textit{negative binomial function}.
This enables a balance between accurate proportional sampling and coverage of sampling.

\section{Parallel Query-Driven ER}
\label{sec:parallelqder}
The previous algorithms described single process sampling over the set of mentions.
The join-driven methods is modeled for several interwoven sequential selection-driven processes.
%To increase performance, sampling can be performed in parallel if a few principles are followed.
In this section, we describe our implementation of the hybrid algorithm over a
parallel database management system.

% Building Vose structre
An independent Vose structure is created for each query node in the query set.
The creation of the Vose structure query nodes is parallelized.
% Scalability limitations
When the number of query nodes increases the Vose structures demand more memory from the system.
Each Vose structure contains array of type double precision and unsigned int.
The space for the structure is $O(|Q|\cdot|M|)$ where $|Q|$ is the number of query nodes in the
query and $|M|$ is the number of mentions in the corpus.
The Vose stucture is accessed over every sample and needs to be in memory.
To increase scalability, instead of storing the full sets of precomputed samlples and offload the 
data Vose Strutures to disk but that is not explore here~\cite {Jampani:2008:MMC:1376616.1376686}.

% Sampling
Sampling over the query nodes for each algorithm can also be perform in parallel.
A thread select a query node using a random schedule as described in Section~ref{sec:jointquery}.
%Other scheduling algorithms would be interesting here
The system will use the Vose structure associated with the query node to set up a proposal move.
The system attempts to obtain a lock for the two entities involved in the proposal.
If the system is unable to obtain a lock on either of the two entities the system will backoff
and resample new entities.
When the number of query nodes is small the query-driven algorithms experience lot of contention
at the entities containing the query nodes.
In these circumstances, the system will backoff and either restart the proposal process or attempt a baseline proposal.
This avoids waiting for locked entities and keeps the sampling process acctive.
In Section~\ref{sec:parallelexperiments} we demonstrate the parallel hybrid method over a large data set.
